# Supplementary material for: Experimental and Phenomenological Investigations of the MiniBooNE Anomaly
Source: arXiv:2308.12015 source file (2023-08-23)
Supplement: Supplementary file 1 [file MBuB_supplemental.pdf]

# Supplemental Materials: MiniBooNE and MicroBooNE Combined Fit to a 3+1 Sterile Neutrino Scenario

## S1. LIKELIHOOD

The physics parameters of the model are the mass squared splitting $\Delta m^2$, electron-sterile mixing $|U_{e4}|^2$, and muon-sterile mixing $|U_{\mu 4}|^2$. The mixing parameters ($|U_{e4}|^2$, $|U_{\mu 4}|^2$) are allowed to vary between 0 and 1 while maintaining unitarity of the mixing matrix through the condition $|U_{e4}|^2 + |U_{\mu 4}|^2 \leq 1$. The additional nuisance parameters of the model are the MicroBooNE per-bin systematic scalings $\alpha_i$. Here the set of physics parameters are denoted by $\vec{\theta}$, and the set of nuisance parameters denoted by $\vec{\eta}$. The combined MiniBooNE-MicroBooNE likelihood is the product the two experimental likelihoods such that

$$\mathcal{L}(\vec{\theta}, \vec{\eta}|\vec{x}) = \mathcal{L}_{\rm MB}(\vec{\theta}|\vec{x}_{\rm MB}) \times \mathcal{L}_{\rm uB}(\vec{\theta}, \vec{\eta}|\vec{x}_{\rm uB}),$$

where $\mathcal{L}_{\rm MB}$ is the MiniBooNE likelihood, $\mathcal{L}_{\rm uB}$ is the MicroBooNE likelihood, $\vec{x}_{\rm MB}$ is collection of the MiniBooNE data counts, $\vec{x}_{\rm uB}$ is the collection of MicroBooNE data counts, and $\vec{x} = \vec{x}_{\rm MB} \cup \vec{x}_{\rm uB}$ is the collection of all data counts. The MiniBooNE likelihood is approximated as a multivariate normal distribution

$$\mathcal{L}_{\rm MB}(\vec{\theta}, \vec{\eta}|\vec{x}_{\rm MB}) = \mathcal{N}(\vec{x}_{\rm MB}|\vec{\mu}_{\rm MB}(\vec{\theta}), \mathbf{\Sigma}_{\rm MB}(\vec{\theta})),$$

where $\vec{\mu}_{\rm MB}$ is the predicted number of data counts in each bin, and $\mathbf{\Sigma}_{\rm MB}$ is the MiniBooNE covariance matrix. In this case the MiniBooNE covariance matrix includes systematic errors, Poisson statistical errors, and Monte-Carlo statistical errors. The MicroBooNE likelihood is given by

$$\mathcal{L}_{\rm uB}(\vec{\theta}, \vec{\eta}|\vec{x}_{\rm uB}) = \mathcal{N}(\vec{\alpha}|1, \mathbf{\Sigma}_{\rm uB}) \times \prod_i \mathcal{L}^{\rm Eff}(\alpha_i \mu_i^{\rm uB}(\vec{\theta}), \sigma^2_{i,\rm mc}(\vec{\theta}, \alpha_i)|x_{i,\rm uB}),$$

where $\mathcal{N}(\vec{\alpha}|1, \mathbf{\Sigma}_{\rm uB})$ is the multivariate normal prior on the MicroBooNE systematics scalings, $\mathbf{\Sigma}_{\rm uB}$ is the MicroBooNE fractional covariance matrix, $\mu_i$ is the predicted number of data counts in each bin before systematic modifications, and $\sigma^2_{i,\rm mc}$ is the Monte-Carlo statistical error on the per-bin data count prediction after the systematics scalings have been applied. The MicroBooNE fractional covariance matrix, $\mathbf{\Sigma}_{\rm uB}$, is the constrained fractional covariance matrix from [1, 2]. The likelihood $\mathcal{L}^{\rm Eff}$ is a Poisson-based likelihood that accounts for finite Monte-Carlo sample errors, and is described in [3]. The minimum $-\log \mathcal{L}$ for each of the 3+1 fit scenarios described in the main text is given in Table S1.

| Datasets Included | $\min_{\vec{\eta}}\{-\log\mathcal{L}\}$ (no-oscillation model) | $\min_{\vec{\theta},\vec{\eta}}\{-\log\mathcal{L}\}$ (3+1 model) |
|---|---|---|
| MiniBooNE only | 219.1 | 205.2 |
| MiniBooNE + DL | 251.0 | 238.7 |
| MiniBooNE + WC | 673.1 | 664.5 |

TABLE S1. Summary of the minimum negative-log-likelihood values for each of the 3+1 fit scenarios described in the main text, including the result for both the no-oscillation and oscillation cases.

## S2. COMBINED FIT WITH MICROBOONE INCLUSIVE ANALYSIS

In this section, we provide the predicted event event rate in the MiniBooNE $\nu_e + \bar{\nu}_e$ and $\nu_\mu + \bar{\nu}_\mu$ distributions, as well as well as the MicroBooNE $\nu_e$ FC, $\nu_e$ PC, $\nu_\mu$ FC and $\nu_\mu$ PC distributions for the "Combination (WC)" best fit to the 3+1 model in Table I. Comparisons between data and prediction in each of these channels is shown in Figure S1. One can see that the best-fit solution prefers negligible $\nu_\mu$ disappearance while still allowing for enough $\nu_\mu(\bar{\nu}_\mu) \to \nu_e(\bar{\nu}_e)$ appearance to explain most of the excess in the MiniBooNE $\nu_e + \bar{\nu}_e$ channel. Additionally, the systematic pull terms in the MicroBooNE analysis modify the prediction in the $\nu_\mu$ FC and $\nu_\mu$ PC channels to match the data, in contrast to the central value prediction shown in Figure 21 of Ref. [4].

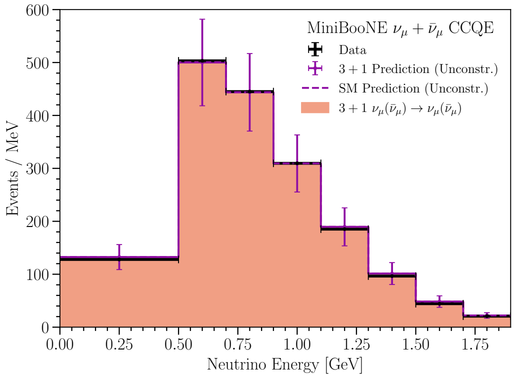


(a) MiniBooNE $\nu_\mu + \bar{\nu}_\mu$

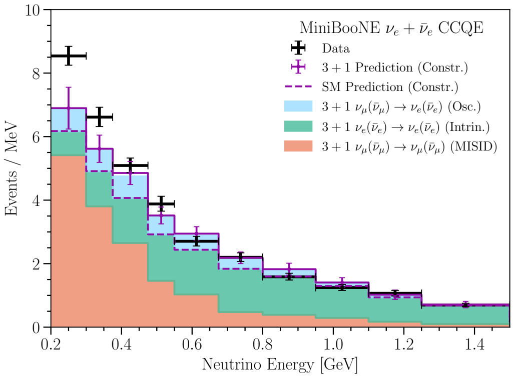


(b) MiniBooNE $\nu_e + \bar{\nu}_e$

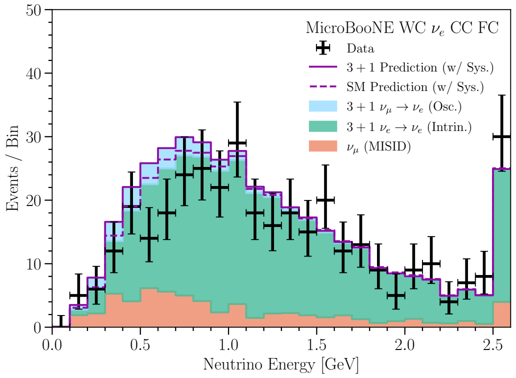


(c) MicroBooNE $\nu_e$ CC FC Inclusive

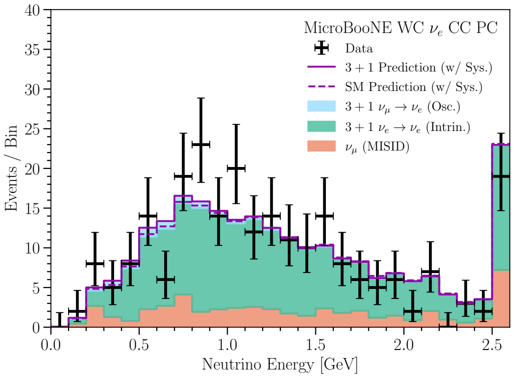


(d) MicroBooNE $\nu_e$ CC PC Inclusive

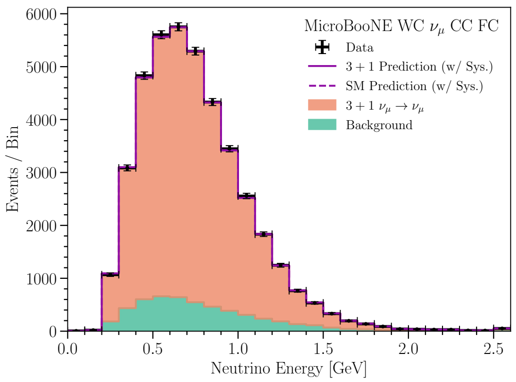


(e) MicroBooNE $\nu_\mu$ CC FC Inclusive

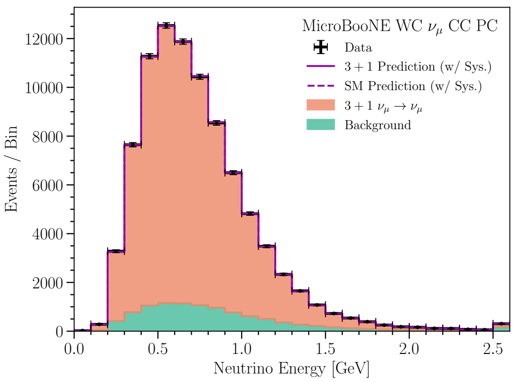


(f) MicroBooNE $\nu_\mu$ CC PC Inclusive

FIG. S1. Comparison between data and prediction for each experiment, showing the prediction from both the SM and the 3+1 model, considering the 3+1 "Combination (WC)" fit parameters of Table I. See the caption of Figure 1 in the main text for a description of the content of each subfigure.

## S3. CONSTRAINTS FROM MICROBOONE DATA

In this section, we report the constraints in 3+1 parameter space derived from each of MicroBooNE samples individually. Results from the CCQE (Inclusive) sample are shown in the left (right) plot of Figure S2. One can see that the Inclusive sample sets a slightly stronger constraint than the CCQE sample.

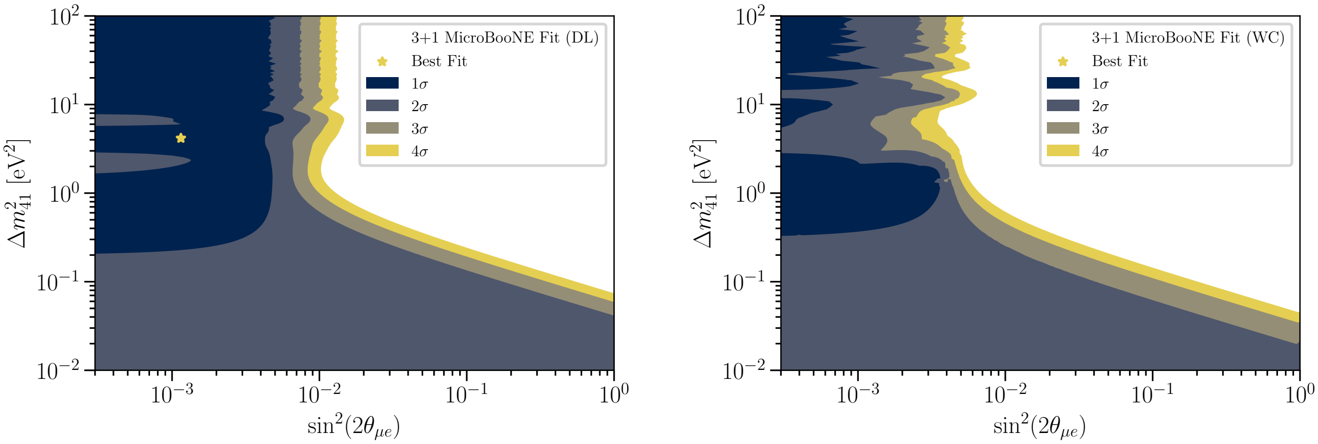


(a) MicroBooNE CCQE Sample

(b) MicroBooNE Inclusive Sample

FIG. S2. Constraints in 3+1 parameter space from the MicroBooNE CCQE (left) and Inclusive (right) samples. See the caption of Figure 2 in the main text for more details on the content shown in each plot. Note that the best fit point for the Inclusive sample lies outside of the window shown here.

---

[S1] P. Abratenko *et al.* (MicroBooNE), Search for an anomalous excess of charged-current quasi-elastic $\nu_e$ interactions with the MicroBooNE experiment using Deep-Learning-based reconstruction, (2021), arXiv:2110.14080 [hep-ex].

[S2] 'NuE background constrained fractional covariance matrix' of 'Search for an anomalous excess of charged-current quasi-elastic $\nu_e$ interactions with the MicroBooNE experiment using Deep-Learning-based reconstruction' (2021).

[S3] C. A. Argüelles, A. Schneider, and T. Yuan, A binned likelihood for stochastic models, JHEP **06**, 030, arXiv:1901.04645 [physics.data-an].

[S4] P. Abratenko *et al.* (MicroBooNE), Search for an anomalous excess of inclusive charged-current $\nu_e$ interactions in the MicroBooNE experiment using Wire-Cell reconstruction, (2021), arXiv:2110.13978 [hep-ex].
